# Supplementary material for: Statistical physics of Bose-Einstein condensed light in a dye microcavity
Source: arXiv:1201.0444 source file (2012-05-15)
Supplement: Supplementary file 1 [file supplemental.pdf]

# Supplemental

**Contents**


**I. Cavity photon dispersion** 2

**II. Thermalization process** 3

A. Kennard-Stepanov law 3

B. Chemical equilibrium 5

C. Rate equations in a microcavity 6

**III. Photon statistics of the condensate** 10

A. Numerical evaluation of $\mathcal{P}_n$ 10

B. Asymptotic photon number distributions 11

C. Crossover of photon statistics 13

D. Second order correlation function $g^{(2)}(\tau)$ 16

**References** 18

## I. CAVITY PHOTON DISPERSION

The photon energy as a function of the longitudinal ($k_z$) and transversal wave number ($k_r$) is

$$E = \hbar\tilde{c}\sqrt{k_z^2 + k_r^2} \; , \tag{S.1}$$

with $\tilde{c}$ as the speed of light in the medium. The resonator boundary conditions in the $z$-direction are incorporated by an ansatz

$$k_z(r) = q\pi/D(r) \; , \tag{S.2}$$

where

$$D(r) = D_0 - 2(R - \sqrt{R^2 - r^2}) \; , \tag{S.3}$$

is the mirror separation at a distance $r$ from the optical axis, $R$ is the radius of curvature and $q$ is the longitudinal excitation number.

In the discussed system, $q$ is assumed to be equal for all photons and not to be altered by the thermalization process [20, 21], i.e. we set $q$ = const. In a paraxial approximation, with $k_r \ll k_z(0)$ and $r \ll R$, this yields

$$\begin{aligned} E &\overset{\text{par.}}{\simeq} \frac{\pi\hbar\tilde{c}q}{D_0} + \frac{\hbar\tilde{c}D_0}{2\pi q}k_r^2 + \frac{\pi\hbar\tilde{c}q}{D_0^2 R}r^2 \\ &= m\tilde{c}^2 + \frac{(\hbar k_r)^2}{2m} + \frac{m\Omega^2}{2}r^2 \; . \end{aligned} \tag{S.4}$$

In the second step we have defined an effective photon mass

$$m = \hbar k_z(0)/\tilde{c} \; , \tag{S.5}$$

and a trap frequency

$$\Omega = \frac{\tilde{c}}{\sqrt{D_0 R/2}} \; , \tag{S.6}$$

to obtain the energy of a 2d harmonic oscillator. The resulting eigenenergy spectrum is $E_{qrs} = E_{q00} + \hbar\Omega\,(r+s)$, with $r$, $s$ as transversal excitation numbers, $E_{q00}$ as transversal ground state energy and a linearly increasing degeneracy of the transversal photon energy, see Fig. 1b of the main text. Thus the photon gas can be mapped onto an atomic (2d) Bose gas in a harmonic trap - a system known to undergo BEC at finite temperatures [1, 2].

## II. THERMALIZATION PROCESS

### A. Kennard-Stepanov law

The Kennard-Stepanov (KS) law relates the spectral profiles of absorption and emission of dye molecules in liquid solution [3–5]. It can either be stated in terms of $A(\omega)/B_{12}(\omega)$ or $B_{21}(\omega)/B_{12}(\omega)$, where $A(\omega)$, $B_{12}(\omega)$ and $B_{21}(\omega)$ are the usual Einstein coefficients of spontaneous emission, absorption and stimulated emission - with the difference being essentially the density of states (A-B relation). The KS relation can be stated in the form

$$\frac{B_{21}(\omega)}{B_{12}(\omega)} = \frac{w_\downarrow}{w_\uparrow} e^{-\frac{\hbar(\omega-\omega_0)}{k_\mathrm{B}T}} \quad , \tag{S.7}$$

where $\omega_0$ is the zero-phonon line of the dye and

$$w_{\downarrow,\uparrow} = \int_{\epsilon\geq 0} \mathcal{D}_{\downarrow,\uparrow}(\epsilon) \exp\left(-\epsilon/k_B T\right)\, d\epsilon \quad , \tag{S.8}$$

are statistical weights related to the rovibronic density of states $\mathcal{D}_{\downarrow,\uparrow}(\epsilon)$ of ground ($\downarrow$) and excited ($\uparrow$) dye state respectively. This law goes back to a thermalization process of the rovibronic dye state due to frequent collisions with solvent molecules. It was discovered at the beginning of the last century [3, 4] and has been rediscovered several times. Both theoretical and experimental investigations can be found in the literature [5–8]. For the sake of completeness, we include a brief derivation in this Supplementary.

As a start, we model the dye molecule an electronic two-level system with levels $S_0$ and $S_1$, here also denoted by $\downarrow$ and $\uparrow$, each of which is subject to additional rovibronic level splitting [9]. The situation is illustrated in the Jablonski diagram given in Fig. 1. It is important to note that the Einstein coefficients of such a medium at a given frequency $\omega$ are an average over all pairs of individual rovibronic substates $(\alpha, \beta)$ with $\alpha \in S_0$, $\beta \in S_1$ that match the transition frequency:

$$e_\alpha + \hbar\omega = \hbar\omega_0 + e_\beta \quad . \tag{S.9}$$

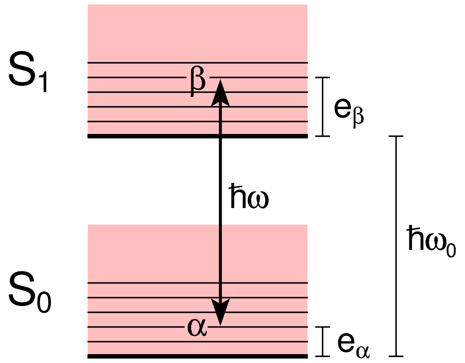


Figure 1: Jablonski diagram of a dye molecule with two electronic levels. Both lower and upper electronic state, $S_0$ and $S_1$, are split into a rovibronic substructure respectively.

Due to frequent collisions with solvent molecules the population of rovibronic states will in very good approximation be thermal, i.e. we assume that every state occurs with a probability according to its Boltzmann factor

$$p_\alpha = e^{-\frac{e_\alpha}{k_B T}}/w_\downarrow \qquad \text{and} \qquad p_\beta = e^{-\frac{e_\beta}{k_B T}}/w_\uparrow \,, \tag{S.10}$$

with the normalization factors

$$w_\downarrow = \sum_{\alpha\in S_0} e^{-\frac{e_\alpha}{k_B T}} \qquad \text{and} \qquad w_\uparrow = \sum_{\beta\in S_1} e^{-\frac{e_\beta}{k_B T}} \quad . \tag{S.11}$$

This will be true for both the $S_0$ and the $S_1$ manifolds, as long as the radiative lifetime of $S_1$, typically nanoseconds, remains longer than the thermalization time which is on a sub-picosecond timescale at room temperature [9]. From eq. (S.9) one immediately obtains

$$\begin{aligned} p_\beta &= \frac{1}{w_\uparrow} e^{-\frac{e_\beta}{k_B T}} \\ &= \frac{1}{w_\uparrow} e^{-\frac{\hbar(\omega-\omega_0)}{k_B T}} e^{-\frac{e_\alpha}{k_B T}} \\ &= \frac{w_\downarrow}{w_\uparrow} e^{-\frac{\hbar(\omega-\omega_0)}{k_B T}} p_\alpha \quad . \end{aligned} \tag{S.12}$$

We can now write

$$\frac{B_{21}(\omega)}{B_{12}(\omega)} = \frac{\sum_{(\alpha,\beta)} p_\beta \, B(\beta\to\alpha)}{\sum_{(\alpha,\beta)} p_\alpha \, B(\alpha\to\beta)} \,, \tag{S.13}$$

where we have introduced the Einstein coefficients $B(\alpha \to \beta)$ for transitions between individual rovibronic states. If one applies $B(\alpha\to\beta) = B(\beta\to\alpha)$ and eq. (S.12), one finally obtains

$$\begin{aligned} \frac{B_{21}(\omega)}{B_{12}(\omega)} &= \frac{w_\downarrow}{w_\uparrow} e^{-\frac{\hbar(\omega-\omega_0)}{k_B T}} \frac{\sum_{(\alpha,\beta)} p_\alpha \, B(\alpha\to\beta)}{\sum_{(\alpha,\beta)} p_\alpha \, B(\alpha\to\beta)} \\ &= \frac{w_\downarrow}{w_\uparrow} e^{-\frac{\hbar(\omega-\omega_0)}{k_B T}} \quad . \end{aligned} \tag{S.14}$$

This yields the Kennard-Stepanov law, see eq. (S.7). The statistical weights can either be expressed as sum over states, as in eq. (S.11), or as integral over a continuous rovibronic density of states, see eq. (S.8).

### B. Chemical equilibrium

By absorption and emission of a photon, the electronic ground state can be excited to the upper electronic level and vice versa. This can be seen as a photochemical reaction of the type

$$\gamma + \downarrow \leftrightharpoons \uparrow \tag{S.15}$$

where $\gamma$ stands for a photon, $\downarrow$ for a molecule in the electronic ground state and $\uparrow$ for a molecule in the excited electronic state. In chemical equilibrium the chemical potentials satisfy the equation [10]

$$\mu_\gamma + \mu_\downarrow = \mu_\uparrow \tag{S.16}$$

so that the photon chemical potential, and likewise the photon fugacity $z$, can be expressed as

$$z = e^{\frac{\mu_\gamma}{k_B T}} = e^{\frac{\mu_\uparrow}{k_B T}} / e^{\frac{\mu_\downarrow}{k_B T}} \ . \tag{S.17}$$

Let the partition function of a dye molecule be

$$\mathcal{F} = w_\downarrow \, e^{\frac{\mu_\downarrow}{k_\mathrm{B} T}} + w_\uparrow \, e^{-\frac{\hbar\omega_0 - \mu_\uparrow}{k_\mathrm{B} T}} \ , \tag{S.18}$$

where $w_{\downarrow,\uparrow} = \int_{\epsilon \geq 0} \mathcal{D}_{\downarrow,\uparrow}(\epsilon) \exp\left(-\epsilon/k_B T\right) \, d\epsilon$ are statistical weights related to the rovibronic density of states $\mathcal{D}_{\downarrow,\uparrow}(\epsilon)$ of ground ($\downarrow$) and excited ($\uparrow$) dye state and $\omega_0$ is the zero-phonon line of the dye. Then we can identify

$$w_\uparrow \, e^{-\frac{\hbar\omega_0 - \mu_\uparrow}{k_\mathrm{B} T}} / \mathcal{F} = \frac{\rho_\uparrow}{\rho} \tag{S.19}$$

$$w_\downarrow \, e^{\frac{\mu_\downarrow}{k_\mathrm{B} T}} / \mathcal{F} = \frac{\rho_\downarrow}{\rho} \tag{S.20}$$

as the probability of finding a molecule in the excited (ground) state, where $\rho_\uparrow$ ($\rho_\downarrow$) is the density of the excited (ground) state dye molecules and $\rho$ is the total density. With this the photon chemical potential, eq. (S.17), is given by

$$z = e^{\frac{\mu_\gamma}{k_\mathrm{B} T}} = \frac{w_\downarrow}{w_\uparrow} \frac{\rho_\uparrow}{\rho_\downarrow} e^{\frac{\hbar\omega_0}{k_B T}} \ . \tag{S.21}$$

In chemical equilibrium, the chemical potential of the photons is thus determined by the excitation ratio $\rho_\uparrow/\rho_\downarrow$ of the dye molecules. For a microresonator environment, as it is investigated here, it proves moreover helpful to define a renormalized chemical potential,

$$\mu := \mu_\gamma - E_{q00} \,, \tag{S.22}$$

by removing the energy of the cavity ground state $E_{q00}$ from all energy quantities. Then we can also write

$$e^{\frac{\mu}{k_{\mathrm{B}}T}} = \frac{w_\downarrow}{w_\uparrow}\frac{\rho_\uparrow}{\rho_\downarrow}\, e^{-\frac{\hbar\Delta}{k_B T}} \,,$$

where we have additionally introduced the dye-cavity detuning, $\Delta = E_{q00}/\hbar - \omega_0$.

### C. Rate equations in a microcavity

In this section, we derive the rate equations of absorption and emission of photons in the microcavity environment, eq. (4) and (5) of the main text. We correspondingly consider a scenario in which the photon emission occurs in an absorbing medium, enclosed in cavity. The light-matter interaction is affected by various cavity specific effects, like spatially inhomogeneous field distributions and Purcell enhancement. Moreover, it is well known that the presence of an absorbing medium has a profound effect on the (spontaneous) emission process, which essentially can be viewed as a consequence of the disrupted self-interference of the photon field in that case [11–13]. We assume the light-matter interaction to be in the weak coupling regime, i.e. the Rabi frequency is assumed to be much smaller than the total dephasing rate, the latter being dominated from collisions with solvent molecules (fs timescale at room temperature [14, 15]).

We first consider the rate of photon emission. Suppose there is an electronically excited dye molecule at cavity position $\mathbf{r}$ that stimulatedly emits into a mode $i$, which is already populated by one photon. The light-matter coupling is described by the coupling parameter of the Jaynes-Cummings Hamiltonian

$$g_i(\mathbf{r}) = \hbar^{-1}\sqrt{\frac{\hbar\omega_i}{2\epsilon_0}}\,\mu\mathbf{d}\cdot\mathbf{f}_i(\mathbf{r}) \,, \tag{S.23}$$

where $\omega_i$ is the frequency of mode $i$, $\mu$ is the dipole strength of the molecular transition, $\mathbf{d}$ is a unity vector describing the dipole orientation and $\mathbf{f}_i(\mathbf{r})$ is the normalized mode function of (one polarization of) mode $i$, with $\int dV\,|\mathbf{f}_i(\mathbf{r})|^2 = 1$.

As usual, we make use of Fermi's golden rule to obtain the transition rate from the initial to the final state

$$\begin{aligned} W_{i\to f} &= 2\pi\,\rho_i(\omega_i)\,|g_i(\mathbf{r})|^2 \\ &= 2\pi\,\rho_i(\omega_i)\,\hbar^{-2}\,\frac{\hbar\omega_i}{2\epsilon_0}\,\mu^2\,|\mathbf{d}\cdot\mathbf{f}_j(\mathbf{r})|^2 \ . \end{aligned} \tag{S.24}$$

In this context, the spectral density of states $\rho_i(\omega)$ is associated to the quasi-mode nature of a cavity resonance, which manifests itself in a finite linewidth. In the literature one often considers systems, in which the finite linewidth is predominantly caused by mirror losses, which differs from the scenario of an ideal cavity that is investigated here. However, it has been noticed before that an absorbing medium inside the cavity essentially has the same effect as lossy mirrors [11–13]. The field in the cavity is determined by the reflections from the mirrors, but an absorbing medium effectively reduces their reflectivities and the overall cavity finesse. This can be incorporated by assuming a finite linewidth $\gamma_i$ for mode $i$. On resonance, $\omega = \omega_i$, one can roughly set $\rho_i(\omega_i) \simeq \gamma_i^{-1}$.

It is no problem to take into account the relative orientation of dipole and mode polarization, which would result in orientation dependent transition rates. However, for the sake of simplicity we remove this degree of freedom by performing a spatial average, $\overline{|\mathbf{d}\cdot\mathbf{f}_i(\mathbf{r})|^2} = \frac{1}{3}\,|f_i(\mathbf{r})|^2$, at this stage of the calculation. The average transition rate is then given by

$$W_{i\to f} = 2\pi\,\rho_i(\omega_i)\,\hbar^{-2}\,\frac{\hbar\omega_i}{2\epsilon_0}\,\mu^2\,\frac{1}{3}|\mathbf{f}_i(\mathbf{r})|^2 \ . \tag{S.25}$$

Finally, if we introduce the spectral energy density per photon in mode $i$ at cavity position $\mathbf{r}$

$$u^i(\mathbf{r}) = \rho_i(\omega_i)\,\hbar\omega_i\,|\mathbf{f}_i(\mathbf{r})|^2 \tag{S.26}$$

and the usual Einstein $B$-coefficient

$$B_{21} = \frac{\pi\mu^2}{3\epsilon_0\hbar^2} \ , \tag{S.27}$$

we can write (S.25) in the familiar form

$$W_{i\to f} = B_{21}\,u^i(\mathbf{r}) \ . \tag{S.28}$$

From eq. (S.28) one can qualitatively conclude that $W_{i\to f}$ will be large, if $u^i(\mathbf{r})$ is large. The energy density $u^i(\mathbf{r})$ itself will be large, if the linewidth $\gamma_i$ is small. Quantitatively, it is easy to see that $u^i(\mathbf{r})$ and $W_{i\to f}$ become enhanced by the

finesse $\mathcal{F}_i$, which is the well known Purcell effect. The Purcell enhancement is mostly discussed in the context of spontaneous emission. However, it equally applies to the rates of stimulated emission and absorption [16, 17].

It is now straightforward to write down the full rate equations, eq. (4) and (5) of the main text. Suppose that the light field $K$ in the cavity is described by a set of mode occupation numbers, $K = (n_0^K, n_1^K, n_2^K, \ldots)$. The corresponding transition rates then are

$$R_{12}^{K,i}(\mathbf{r}) \;=\; B_{12}(\omega_i)\, u^i(\mathbf{r})\, \rho_\downarrow\, n_i^K \tag{S.29}$$

$$R_{21}^{K,i}(\mathbf{r}) \;=\; B_{21}(\omega_i)\, u^i(\mathbf{r})\, \rho_\uparrow\, (n_i^K{+}1)\ , \tag{S.30}$$

where $R_{12}^{K,i}(\mathbf{r})$, $R_{21}^{K,i}(\mathbf{r})$ are the rates per volume of absorbing and emitting a photon in mode $i$ at cavity position $\mathbf{r}$ (the term $+1$ in eq. (S.30) corresponds to spontaneous emission). As we use molecular number densities of excited and ground state molecules $\rho_{\uparrow,\downarrow}$ on the right hand side of eq. (S.29) and (S.30), we obtain rates per volume on the left hand side. The total rates would be given by an integral over the volume. In the main text we show that under certain conditions the rate equations (S.29), (S.30) fulfill a detailed balance condition, which guarantees the thermalization of the light field after repeated absorption-emission cycles.

In the master equation governing the probability flow of the condensate photon number

$$\dot{p}_n = R_{n-1}^{21}\, p_{n-1} - (R_n^{12}{+}R_n^{21})\, p_n + R_{n+1}^{12}\, p_{n+1}\ , \tag{S.31}$$

eq. (9) of the main text, we use absorption and emission rates

$$R_n^{12} \;=\; \hat{B}_{12} M_\downarrow^n n \tag{S.32}$$

$$R_n^{21} \;=\; \hat{B}_{21} M_\uparrow^n (n{+}1)\ , \tag{S.33}$$

where $M_\uparrow^n = X - n$ is the number of excited and $M_\downarrow^n = M - X + n$ the number of ground state molecules respectively, if there are $n$ photons, $X$ (molecular and photonic) excitations and $M$ dye molecules in the volume of the cavity ground state ($X$ and $M$ are treated as fixed parameters in our calculations, see below). These rates follow from eq. (S.29) and (S.30) by an integral over the cavity volume. For example, if one specifies $i = q00$, $\omega_i = E_{q00}/\hbar$ and $n_i^K = n$, then

the absorption rate becomes

$$\begin{aligned} R_n^{12} &= \int dV\, R_{12}^{K,i}(\mathbf{r}) \\ &= \int dV\, B_{12}(E_{q00}/\hbar)\, u^{q00}(\mathbf{r})\, \rho_\downarrow^n\, n \\ &= B_{12}(E_{q00}/\hbar)\, u^{q00}(\mathbf{0})\, n\, \rho_\downarrow^n \int dV\, \frac{|f^{q00}(\mathbf{r})|^2}{|f^{q00}(\mathbf{0})|^2}\ . \end{aligned} \tag{S.34}$$

In the last step we have used $u^{q00}(\mathbf{r}) = u^{q00}(\mathbf{0}) \cdot |f^{q00}(\mathbf{r})|^2/|f^{q00}(\mathbf{0})|^2$. With the effective mode volume $V_{\text{eff}}^{q00}$ defined analogously to [18],

$$V_{\text{eff}}^{q00} = \int dV\, \frac{|f^{q00}(\mathbf{r})|^2}{\mathbf{max}\,\{|f^{q00}(\mathbf{r})|^2\}} = \int dV\, \frac{|f^{q00}(\mathbf{r})|^2}{|f^{q00}(\mathbf{0})|^2} = \frac{1}{|f^{q00}(\mathbf{0})|^2}\ , \tag{S.35}$$

we arrive at

$$\begin{aligned} R_n^{12} &= B_{12}(E_{q00}/\hbar)\, u^{q00}(\mathbf{0})\, n\, \rho_\downarrow^n\, V_{\text{eff}}^{q00} \\ &= \hat{B}_{12}\, n\, M_\downarrow^n\ , \end{aligned} \tag{S.36}$$

if we define $\hat{B}_{12} := B_{12}\, u^{q00}(\mathbf{0})$ and $M_\downarrow^n := \rho_\downarrow^n\, V_{\text{eff}}^{q00}$.

The master equation eq. (S.31) contains two simplifications. Both the number of dye molecules in the ground mode volume $M$ and the total number of excitations in the ground mode volume $X$ are expected to be constant, i.e. $M = \text{const}$ and $X = \text{const}$. Clearly, both assumptions can only approximately be true. For example, the dye molecules may diffuse in the solvent and therefore can enter and leave the ground mode volume. Thus $M$ will fluctuate in time around its mean value. The same holds for $X$; photons can be emitted to (and be absorbed from) higher transversal modes. However, we neither expect $M$ nor $X$ to show fluctuations of order 100%, i.e. neither the number of dye molecules nor the number of excitations in the ground mode volume can be expected to go to zero at a certain point in time. Many uncorrelated events contribute to these diffusion processes and most likely mutually cancel out each other. We expect the fluctuations in $M$ and $X$ to be small in the sense of our letter and therefore neglect them. In any case, taking them into account would only increase the number fluctuations of the ground mode.

## III. PHOTON STATISTICS OF THE CONDENSATE

### A. Numerical evaluation of $\mathcal{P}_n$

In this section we describe the procedure used to numerically evaluate the photon number distribution of the cavity ground state, see eq. (10) of the main text

$$\frac{\mathcal{P}_n}{\mathcal{P}_0} = \frac{(M-X)!\,X!}{(M-X+n)!\,(X-n)!}\left(\frac{\hat{B}_{21}}{\hat{B}_{12}}\right)^n . \tag{S.37}$$

We consider experimental conditions where the temperature is varied, while the average total photon number in the cavity is fixed, i.e. $\bar{N} = \text{const}$. Correspondingly, for each temperature value $T$ we first have to derive the excitation number $X$ that preserves $\bar{N}$.

Our calculation proceeds as follows. For a given test value of $X$, the average ground state occupation

$$\bar{n}_0 = \sum_{n\geq 0} n\mathcal{P}_n , \tag{S.38}$$

is calculated, which also yields the average molecular excitation level of the medium in the ground state volume,

$$\frac{\rho_\uparrow}{\rho_\downarrow} = \frac{X-\bar{n}_0}{M-X+\bar{n}_0} . \tag{S.39}$$

We assume chemical equilibrium between photons, ground state and excited molecules, which is expressed by eq. (S.21). This equation implies that the excitation level in the medium has to be spatially homogeneous, as otherwise gradients in the chemical potential would occur, which are not allowed in equilibrium. Correspondingly, the excitation level determined for the volume of the ground mode eq. (S.39) already gives the excitation level at all other cavity positions. With eq. (S.21), the obtained value for the ratio $\rho_\uparrow/\rho_\downarrow$ is then converted into the photon chemical potential $\mu_\gamma$, which is used to derive the average photon number contribution $\bar{n}_{\text{exc}}$ from the transversally excited modes via

$$\bar{n}_{\text{exc}} = \sum_{u>0} \frac{g(u)}{e^{\frac{E_{q00}+u-\mu_\gamma}{k_{\mathrm{B}}T}} - 1} . \tag{S.40}$$

Here we use the grandcanonical expression for the average occupation of the excited resonator levels. This is justified because the average occupation of a transversally excited mode is always small enough to consider the excitation exchange with its dye molecule reservoir as grandcanonical. If the sum $\bar{n}_0+\bar{n}_{\text{exc}}$ differs from the given 'target' photon number $\bar{N}$, we readjust our value of $X$ accordingly. This procedure is repeated until a given level of precision is reached.

### B. Asymptotic photon number distributions

In this section, we discuss the limiting cases of the photon number distribution obtained in the main text. Expressed in terms of $\mathcal{P}_n$ and $\mathcal{P}_{n+1}$ this distribution can be written as

$$\frac{\mathcal{P}_{n+1}}{\mathcal{P}_n} = \frac{X-n}{M-X+n+1}\frac{\hat{B}_{21}}{\hat{B}_{12}} \ . \tag{S.41}$$

**Bose-Einstein distribution** - The photon statistics will be Bose-Einstein-like, if $\mathcal{P}_n$ is given by a geometric sequence. For that, the ratio $\mathcal{P}_{n+1}/\mathcal{P}_n$ has to be independent of $n$. This will be the case, if the molecular reservoir ($M$, $X$) is so large, that $n$ can be neglected on the right hand side of eq. (S.41) (grandcanonical limit). Then $X \simeq M_\uparrow$ and $M-X \simeq M_\downarrow$, and one obtains

$$\frac{\mathcal{P}_{n+1}}{\mathcal{P}_n} \overset{gr.can.}{=} \frac{\bar{M}_\uparrow}{\bar{M}_\downarrow}\frac{\hat{B}_{21}}{\hat{B}_{12}} \quad \Longrightarrow \quad \frac{\mathcal{P}_n}{\mathcal{P}_0} \overset{gr.can.}{=} \left(\frac{\bar{M}_\uparrow}{\bar{M}_\downarrow}\frac{\hat{B}_{21}}{\hat{B}_{12}}\right)^n \ . \tag{S.42}$$

Thus, $\mathcal{P}_n$ here decays exponentially starting from a maximum value at $n=0$. After normalizing, this distribution can also be written as

$$\mathcal{P}_n = \left(\frac{\bar{M}_\uparrow}{\bar{M}_\downarrow}\frac{\hat{B}_{21}}{\hat{B}_{12}} - 1\right)\left(\frac{\bar{M}_\uparrow}{\bar{M}_\downarrow}\frac{\hat{B}_{21}}{\hat{B}_{12}}\right)^n \tag{S.43}$$

$$= \frac{\left(\frac{\bar{n}_0}{\bar{n}_0+1}\right)^n}{\bar{n}_0+1} \tag{S.44}$$

with an average condensate occupation $\bar{n}_0 = \Big((M_\downarrow \hat{B}_{12}/M_\uparrow \hat{B}_{21}) - 1\Big)^{-1}$.

**Poisson distribution** - If $\mathcal{P}_n$ is not Bose-Einstein-distributed, it has a most probable photon number at a nonzero value $n_{\max}$, which to good approximation can be found by solving the relation $\mathcal{P}_{n_{\max}+1} = \mathcal{P}_{n_{\max}}$. With eq. (S.41) we readily derive

$$n_{\max} = X - \frac{M+1}{\hat{B}_{21}/\hat{B}_{12}+1} \ . \tag{S.45}$$

For further evaluation, we now develop $\mathcal{P}_{n+1}/\mathcal{P}_n$, see eq. (S.41), around $n{=}n_{\rm max}$:

$$\frac{\mathcal{P}_{n+1}}{\mathcal{P}_n} = 1 - \frac{\Delta n}{\lambda} + \frac{\left(\frac{\Delta n}{\lambda}\right)^2}{\left(\hat{B}_{21}/\hat{B}_{12}{+}1\right)} - \frac{\left(\frac{\Delta n}{\lambda}\right)^3}{\left(\hat{B}_{21}/\hat{B}_{12}{+}1\right)^2} + \ldots \tag{S.46}$$

Here $\Delta n = n - n_{\rm max}$ is the deviation from the maximum, and the parameter $\lambda$ is given by

$$\lambda = \frac{\hat{B}_{21}}{\hat{B}_{12}} \frac{M{+}1}{(\hat{B}_{21}/\hat{B}_{12}{+}1)^2} \ . \tag{S.47}$$

We now discuss the low temperature limit ($T \to 0$). In this case we have

$$\frac{\hat{B}_{21}}{\hat{B}_{12}} = \frac{w_\downarrow}{w_\uparrow} e^{-\frac{\hbar\Delta}{k_{\rm B}T}} \overset{T\to 0}{\simeq} \begin{cases} 0 & \Delta{>}0 \\ \infty & \Delta{<}0 \end{cases} . \tag{S.48}$$

Thus, for $\mathcal{P}_{n+1}/\mathcal{P}_n$, as given in eq. (S.46), one asymptotically obtains:

$$\begin{aligned} \frac{\mathcal{P}_{n+1}}{\mathcal{P}_n} &\overset{T\to 0}{\simeq} \begin{cases} 1 - \frac{\Delta n}{\lambda} + \left(\frac{\Delta n}{\lambda}\right)^2 - \left(\frac{\Delta n}{\lambda}\right)^3 + \ldots & \Delta{>}0 \\ 1 - \frac{\Delta n}{\lambda} & \Delta{<}0 \end{cases} \\ &= \begin{cases} \frac{\lambda}{\lambda+\Delta n} & \Delta{>}0 \\ \frac{\lambda-\Delta n}{\lambda} & \Delta{<}0 \end{cases} \end{aligned} \tag{S.49}$$

With this, $\mathcal{P}_n$ can now be written in the form

$$\frac{\mathcal{P}_{n_{\rm max}+\Delta n}}{\mathcal{P}_{n_{\rm max}}} \overset{T\to 0}{\simeq} \begin{cases} \frac{(\lambda-1)!}{(\lambda-1+\Delta n)!}\,\lambda^{\Delta n} & \Delta{>}0 \\ \frac{\lambda!}{(\lambda-\Delta n)!}\,\lambda^{-\Delta n} & \Delta{<}0 \ . \end{cases} \tag{S.50}$$

For both cases one finds essentially the same photon number distribution. The only noteworthy difference is that the distribution for negative detuning, $\Delta{<}0$, is mirrored around the maximum, $\Delta n \to -\Delta n$. Both distributions are basically Poisson-like. This can be seen if one determines $\mathcal{P}_{n_{\rm max}+\Delta n}/\mathcal{P}_{n_{\rm max}}$ for a usual Poisson distribution, $\mathcal{P}_n = e^{-\lambda}\lambda^n/n!$, which yields the same expression as given by eq. (S.49) for the case $\Delta > 0$. We point out that the obtained distributions are Poisson-like only as a function of the relative photon number $\Delta n$. Compared to a true Poisson distribution, they contain a shift in the absolute photon number. This additional degree of freedom is reflected by two different parameters, $n_{\rm max}$ and $\lambda$. For a usual Poisson distribution both parameters are identical, but in our case they can differ. For example, in the extreme limit $T = 0$ and a non-zero dye cavity detuning $\Delta \neq 0$, one finds $n_{\rm max} = n_0 = \bar{N}$ and $\lambda = 0$, meaning that all photons occupy the ground state and the condensate number becomes sharply defined.

### C. Crossover of photon statistics

As done in the main text, we will at first disregard the two-fold polarization degeneracy of the resonator modes. In this case, the BEC phase transition occurs at

$$T_{\rm c}^{(\rm n.deg.)} = \frac{\sqrt{6}\hbar\Omega}{\pi k_{\rm B}}\sqrt{\bar{N}} = \frac{2\sqrt{3}\hbar\tilde{c}}{\pi k_{\rm B}}\sqrt{\frac{1}{D_0}\frac{\bar{N}}{R}} \ . \tag{S.51}$$

For the crossover from Bose-Einstein to Poisson photon statistics, it is a natural choice to consider the point at which having 'zero photons' is no longer the most probable case for the cavity ground state. This occurs for $\mathcal{P}_0 = \mathcal{P}_1$, which using eq. (S.41) can be written as

$$\frac{M+1}{X} = 1 + \frac{\hat{B}_{21}}{\hat{B}_{12}} \ . \tag{S.52}$$

In the following $M \gg 1$ is assumed, so that one can safely set $M{+}1 \simeq M$. We aim at a determination of the corresponding temperature $T_x$ for experimental conditions where the system size $\bar{N}$ (total average photon number) and the reservoir size $M$ are fixed parameters.

We calculate the ground state occupation at which eq. (S.52) is reached. Substituting $X = \bar{M}_\uparrow + \bar{n}_0$ in eq. (S.52), and solving for $\bar{n}_0$ yields

$$\bar{n}_0 = M\left(\left(1+\frac{\hat{B}_{21}}{\hat{B}_{12}}\right)^{-1} - \frac{\bar{M}_\uparrow}{M}\right) \ . \tag{S.53}$$

By further substituting $M = \bar{M}_\uparrow + \bar{M}_\downarrow$, one obtains

$$\bar{n}_0 = M\left(\left(1+\frac{\hat{B}_{21}}{\hat{B}_{12}}\right)^{-1} - \left(1+\frac{\bar{M}_\downarrow}{\bar{M}_\uparrow}\right)^{-1}\right) \tag{S.54}$$

$$= M\,\frac{\frac{\hat{B}_{12}}{\hat{B}_{21}}\frac{\bar{M}_\downarrow}{\bar{M}_\uparrow} - 1}{\left(1+\frac{\hat{B}_{12}}{\hat{B}_{21}}\right)\left(1+\frac{\bar{M}_\downarrow}{\bar{M}_\uparrow}\right)} \tag{S.55}$$

The nominator in eq. (S.55) is the inverse grandcanonical expression for $\bar{n}_0$:

$$\bar{n}_0 = \sum_{n=0}^{\infty} n\mathcal{P}_n \overset{gr.can.}{=} \left(\frac{\hat{B}_{12}}{\hat{B}_{21}}\frac{\bar{M}_\downarrow}{\bar{M}_\uparrow} - 1\right)^{-1} = \left(e^{\frac{E_{q00}-\mu_\gamma}{k_{\rm B}T}} - 1\right)^{-1} \ . \tag{S.56}$$

This is exact only if the sum in eq. (S.56) contains a geometric series, $\mathcal{P}_n \propto (\hat{B}_{21}\bar{M}_\uparrow/\hat{B}_{12}\bar{M}_\downarrow)^n$, which, strictly speaking, only holds if the photon exchange with the ground state does not significantly perturb the excitation level $\bar{M}_\uparrow/\bar{M}_\downarrow$ of the medium. For that $\bar{M}_\uparrow$ and $\bar{M}_\downarrow$ have to be sufficiently large (grandcanonical

limit). At the boundary between fluctuating and non-fluctuating condensate, which we here aim at, this is not perfectly true anymore. However, we still expect it to give an accurate approximation for $\bar{n}_0$, which is also numerically verified later. Thus, using the approximate substitution eq. (S.56) and again solving for $\bar{n}_0$ yields

$$\bar{n}_0 \simeq \sqrt{\frac{M}{\left(1+\frac{\hat{B}_{12}}{\hat{B}_{21}}\right)\left(1+\frac{\bar{M}_\downarrow}{\bar{M}_\uparrow}\right)}} = \sqrt{\frac{M}{\left(1+\frac{w_\uparrow}{w_\downarrow}e^{\frac{\hbar\Delta}{k_\mathrm{B}T}}\right)\left(1+\frac{w_\downarrow}{w_\uparrow}e^{\frac{\hbar\omega_0-\mu_\gamma}{k_B T}}\right)}} \ , \tag{S.57}$$

where in the second step we have employed the KS relation, see eq. 2 of the main text, assumed chemical equilibrium, see eq. 3, and used the dye-cavity detuning $\Delta = E_{q00}/\hbar - \omega_0$. For $T < T_\mathrm{c}$ the chemical potential of the photons is in the range $E_{q00} - \hbar\Omega \leq \mu_\gamma \leq E_{q00}$, with $\hbar\Omega \ll E_{q00}$. We can safely set $\mu_\gamma \simeq E_{q00}$ in eq. (S.57). The reduced chemical potential $\mu$ is then close to zero. Equation (S.57) delivers an upper bound for the ground state occupation up to which the photon statistics can considered to be Bose-Einstein-like. The associated temperature $T_\mathrm{x}$ is implicitly given by the solution of the transcendental equation

$$\bar{N}\left(1-\left(T_\mathrm{x}/T_\mathrm{c}\right)^2\right) \simeq \sqrt{\frac{M}{\left(1+\frac{w_\uparrow}{w_\downarrow}e^{\frac{\hbar\Delta}{k_\mathrm{B}T_\mathrm{x}}}\right)\left(1+\frac{w_\downarrow}{w_\uparrow}e^{-\frac{\hbar\Delta}{k_\mathrm{B}T_\mathrm{x}}}\right)}} \ , \tag{S.58}$$

where we used $\bar{n}_0 = \bar{N}\left(1-\left(T_\mathrm{x}/T_\mathrm{c}\right)^2\right)$ as the ground state occupation. The statistical weights $w_\uparrow$, $w_\downarrow$ due to the rovibronic density of states of the dye molecules in the electronic excited and ground state respectively are not expected to differ strongly from each other and for the sake of simplicity we assume $w_\downarrow = w_\uparrow$. This has been done to obtain eq. 11 of the main text, where we additionally have used eq. (S.51) to specify the critical temperature.

To study the scaling properties of the reduced crossover temperature $t = T_\mathrm{x}/T_\mathrm{c}$ with the system parameters, we rewrite eq. (S.58) in the form

$$1-t^2 \simeq \frac{\sqrt{M}}{\bar{N}}\left(\left(1+e^{\frac{\hbar\Delta}{k_\mathrm{B}T_\mathrm{c}}\frac{1}{t}}\right)\left(1+e^{-\frac{\hbar\Delta}{k_\mathrm{B}T_\mathrm{c}}\frac{1}{t}}\right)\right)^{-\frac{1}{2}} \ . \tag{S.59}$$

One finds that $t$ depends only on two parameters, the system size ratio $\sqrt{M}/\bar{N}$ and the reduced dye-cavity detuning $\hbar\Delta/k_\mathrm{B}T_\mathrm{c}$. This is important when considering the thermodynamic limit, because we now can exclude that $T_\mathrm{x}$ differs from $T_\mathrm{c}$ only due to finite system size. This is clearly not the case if the thermodynamic limit is performed in the following way:

$$\bar{N}, R, M \to \infty \quad \text{with} \quad \frac{R}{\bar{N}} = \text{const} \quad \text{and} \quad \frac{\sqrt{M}}{\bar{N}} = \text{const} \ . \tag{S.60}$$

The first constraint $R/\bar{N}=\text{const}$ ($R$ radius of curvature) conserves $T_\text{c}$, see eq. (S.51); and also fixes the reduced dye-cavity detuning $\hbar\Delta/k_\text{B}T_\text{c}$. The second constraint $\sqrt{M}/\bar{N}=\text{const}$ then leads to the conservation of $T_\text{x}$ at a value below $T_\text{c}$. Thus, we conclude that $T_\text{x}$can differ from $T_\text{c}$ also in the thermodynamic limit.

We have performed a consistency check between the analytic approximation eq. (S.58) and our numerical exact calculations based on the direct evaluation of the probability distribution $\mathcal{P}_n$, which are given in Fig. 2 of the main text. For that, we have numerically determined the temperature at which $\mathcal{P}_0=\mathcal{P}_1$ in a system with $\bar{N}=10^4$ photons, six different reservoir sizes ranging from $M_1=10^8$ up to $M_6=10^{13}$ and a reduced dye-cavity detuning of $\hbar\Delta/k_\text{B}T_\text{c}=-4.35$. The corresponding values can be found in the table below:

| | $M_1=10^8$ | $M_2=10^9$ | $M_3=10^{10}$ | $M_4=10^{11}$ | $M_5=10^{12}$ | $M_6=10^{13}$ |
|---|---|---|---|---|---|---|
| $T_\text{x}/T_\text{c}$ [num.] | 0.9444 | 0.8737 | 0.7421 | 0.5900 | 0.4679 | 0.3812 |
| $T_\text{x}/T_\text{c}$ [ana.] | 0.9486 | 0.8638 | 0.7182 | 0.5659 | 0.4498 | 0.3681 |
| Deviation | +0.44% | -1.1% | -3.2% | -4.1% | -3.9% | -3.4% |
| $g^{(2)}(0)$ [num.] | 1.569956 | 1.570477 | 1.570640 | 1.570691 | 1.570709 | 1.570717 |
| $\bar{n}_0/\bar{N}$ [num.] | 0.079 | 0.208 | 0.426 | 0.634 | 0.768 | 0.844 |

The first two lines contain the reduced crossover temperatures obtained by the numerical exact evaluation of $\mathcal{P}_n$ ('num.') and the analytic approximation eq. (S.58) ('ana.'), respectively. The third line gives the deviation between the two values, which is never above a few percent. We have moreover included corresponding values for the second order correlation function and the condensate fraction at $\mathcal{P}_0=\mathcal{P}_1$. We find $g^{(2)}(0)\simeq 1.571$, being notably close to $\pi/2$, and condensate fractions ranging from 8% for the smallest reservoir $M_1$ to 84% for the largest reservoir $M_6$.

Finally, we discuss the modifications if the two-fold polarization degeneracy of the resonator modes is considered, which corresponds to the experimental situation in [19–21]. The BEC phase transition temperature here is a factor $\sqrt{2}$ larger than in the non-degenerate case and is given by

$$T_\text{c}^{(\text{deg.})}=\frac{\sqrt{3}\hbar\Omega}{\pi k_\text{B}}\sqrt{\bar{N}}=\frac{\sqrt{6}\hbar\tilde{c}}{\pi k_\text{B}}\sqrt{\frac{1}{D_0}\frac{\bar{N}}{R}}\ . \tag{S.61}$$

For a description of the photon statistics in the polarization degenerate case, it is necessary to consider a two-dimensional probability distribution $\mathcal{P}_{n,m}$, which denotes the probability to simultaneously find $n$ photons of polarization 1 and $m$ photons of polarization 2 in the energetic ground state. The conservation of excitations now requires $X = M_{\uparrow}^{n,m} + n + m = \text{const}$, with $M_{\uparrow}^{n,m}$ as the number of excited molecules. The corresponding master equation contains additional terms, but can still be solved analytically (except for normalization). Let us skip the details, and directly move to a discussion of the photon statistics crossover.

Similarly as above, there is no unique choice for the border between Bose-Einstein and Poisson statistics. It is however natural to consider the photon number distribution as being Bose-Einstein-like as long as $\mathcal{P}_{0,0}$ is the maximum of the distribution. This holds until

$$\mathcal{P}_{0,0} = \mathcal{P}_{1,0} = \mathcal{P}_{0,1} \tag{S.62}$$

is reached, which gives exactly the same crossover condition as above, see eq. (S.52). Thus, the polarization degeneracy does not qualitatively change the situation. The associated temperature $T_{\mathrm{x}}$ is given by the solution of

$$\frac{\bar{N}}{2}\left(1-\left(T_{\mathrm{x}}/T_{\mathrm{c}}\right)^2\right) \simeq \sqrt{\frac{M}{\left(1+\frac{w_\uparrow}{w_\downarrow}e^{\frac{\hbar\Delta}{k_{\mathrm{B}}T_{\mathrm{x}}}}\right)\left(1+\frac{w_\downarrow}{w_\uparrow}e^{-\frac{\hbar\Delta}{k_{\mathrm{B}}T_{\mathrm{x}}}}\right)}}\,. \tag{S.63}$$

Compared to eq. (S.58), an additional factor of 1/2 arises due to the splitting of the ground state occupation into two polarization modes, and $T_{\mathrm{c}}$ differing by a factor $\sqrt{2}$.

### D. Second order correlation function $g^{(2)}(\tau)$

In this section, we aim at a determination of the second order correlation function of a fluctuating condensate. As above, we first disregard the two-fold polarization degeneracy, and discuss modifications due to this degeneracy at the end of the section. The calculation is performed in two steps. We first determine the relaxation time of the ground state population that is required to return to its average value when starting from a given initial value. In a second step, an average over all initial values is performed.

To determine the time evolution of the average ground mode occupation $\bar{n}_0(t) = \sum_{n=0}^{\infty} n\, p_n(t)$ for given initial conditions $p_n(0) = \delta_{n,n_{\mathrm{i}}}$ (resulting in

$\bar{n}_0(0)=n_{0,\mathrm{i}}$), we solve the time-dependent master equation for the diagonal elements $p_n=p_n(t)$ of the density matrix

$$\dot{p}_n = R^{21}_{n-1}\,p_{n-1} - (R^{12}_n+R^{21}_n)\,p_n + R^{12}_{n+1}\,p_{n+1} \tag{S.64}$$

where the rates are a function of the photon number $n$, and given by

$$R^{12}_n \;=\; \hat{B}_{12}M_{\downarrow}n \tag{S.65}$$

$$R^{21}_n \;=\; \hat{B}_{21}M_{\uparrow}(n+1)\ . \tag{S.66}$$

We restrict the discussion to the regime of large reservoir sizes, corresponding to the grandcanonical limit (for which the condensate number fluctuations are large). The reservoir sizes $M_{\downarrow,\uparrow}$ are considered as fixed parameters, which are not affected by the photon exchange with the resonator ground state. For our calculation, the generating function technique is used [22]. The generating function $F(z,t)$ is defined as

$$F(z,t) = \sum_{n=0}^{\infty} p_n(t)\, z^n\ . \tag{S.67}$$

If the time evolution of $p_n(t)$ is governed by eq. (S.64), $F(z,t)$ will fulfill the partial differential equation

$$\frac{\partial F(z,t)}{\partial t} = \Big(\big(z^{-1}-1\big)\, R^{12}_n[n\rightarrow z\partial_z] + (z-1)\ R^{21}_n[n\rightarrow z\partial_z]\Big)\, F(z,t)\ , \tag{S.68}$$

(and vice versa) where the differential operators $R^{12,21}_n[n\rightarrow z\partial_z]$ are obtained by substituting $n$ with $z\partial_z$ in eq. (S.65), (S.66):

$$R^{12}_n[n\rightarrow z\partial_z] \;=\; \hat{B}_{12}M_{\downarrow}z\partial_z \tag{S.69}$$

$$R^{21}_n[n\rightarrow z\partial_z] \;=\; \hat{B}_{21}M_{\uparrow}(z\partial_z+1)\ . \tag{S.70}$$

The generating function $F(z,t)$ is related to the time-dependent $k$-th momentum of the ground state occupation $\langle n_0^k(t)\rangle$ by

$$\langle n_0^k(t)\rangle = \Big[\big(z\partial_z\big)^k F(z,t)\Big]_{z=1}\ . \tag{S.71}$$

We specify initial conditions by assuming to have with certainty $n_{0,\mathrm{i}}$ photons in the ground state at $t=0$, which corresponds to $F(z,0)=z^{n_{0,\mathrm{i}}}$. The solution of eq. (S.68) for these initial conditions is found to be

$$F(z,t) = \frac{\left(1 + \frac{e^{-t/\tau_c^{(2)}}(z-1)}{1+\bar{n}_0(e^{-t/\tau_c^{(2)}}-1)\,(z-1)}\right)^{n_\mathrm{i}}}{1+\bar{n}_0\,(e^{-t/\tau_c^{(2)}}-1)\,(z-1)}\ , \tag{S.72}$$

where we have already incorporated the asymptotic ground state occupation

$$\bar{n}_0 = \bar{n}_0(\infty) = \frac{1}{\hat{B}_{12}M_\downarrow/\hat{B}_{21}M_\uparrow - 1} \tag{S.73}$$

and defined the decay time $\tau_c^{(2)} = \bar{n}_0/\hat{B}_{21}M_\uparrow$. Using eq. (S.71) for $k=1$ now results in

$$\bar{n}_0(t) = \bar{n}_0 + (n_{0,\mathrm{i}} - \bar{n}_0)\, e^{-t/\tau_c^{(2)}} \ . \tag{S.74}$$

Thus, an initial ground state population $n_{0,\mathrm{i}}$ decays exponentially with time into equilibrium with a decay time constant $\tau_c^{(2)}$. The second order correlation function is obtained using a weighted average over all initial populations $n_{0,\mathrm{i}}$

$$g^{(2)}(\tau) \ = \ \frac{\langle n_0(0) \times (n_0(\tau) - 1)\rangle}{\bar{n}_0^2} \tag{S.75}$$

$$= \ \bar{n}_0^{-2} \sum_{n_{0,\mathrm{i}}=0}^{\infty} \mathcal{P}_{n_{0,\mathrm{i}}}\, n_{0,\mathrm{i}} \times (\bar{n}_0 + (n_{0,\mathrm{i}} - \bar{n}_0)\, e^{-t/\tau_c} - 1) \ , \tag{S.76}$$

where $\mathcal{P}_{n_\mathrm{i}} := p_{n_\mathrm{i}}(\infty)$ is given by the Bose-Einstein distribution

$$\mathcal{P}_{n_{0,\mathrm{i}}} = \frac{\left(\frac{\bar{n}_0}{\bar{n}_0+1}\right)^{n_{0,\mathrm{i}}}}{\bar{n}_0 + 1} \ .$$

Finally, this results in

$$g^{(2)}(\tau) \ = \ 1 + e^{-\tau/\tau_c^{(2)}} \ . \tag{S.77}$$

Thus, starting from $g^{(2)}(0) = 2$, the second order correlations decay exponentially in time with a correlation time

$$\tau_c^{(2)} = \frac{\bar{n}_0}{\hat{B}_{21}M_\uparrow} \ , \tag{S.78}$$

being proportional to the average condensate number $\bar{n}_0$ and inversely proportional to the number of excited dye molecules $M_\uparrow$. In the grandcanonical regime one can also set $M_\uparrow \simeq X$, which yields $\tau_c^{(2)} = \bar{n}_0/\hat{B}_{21}X$.

Finally, we consider the case of a two-fold polarization degeneracy of modes. Due to the uncorrelated contributions from the two different modes, the autocorrelation function of the fluctuating condensate now starts at a zero-delay value of $g^{(2)}(0) = 3/2$. In an experiment detecting only light with a single polarization, one would nevertheless expect to observe a value of $g^{(2)}(0) = 2$.

---

[1] V. Bagnato and D. Kleppner, Phys. Rev. A **44**, 7439 (1991).

[2] T. Haugset, H. Haugerud, and J.O. Andersen, Phys. Rev. **A** 55, 2922 (1997).

[3] E.H. Kennard, Phys. Rev. **11**, 29 (1918).

[4] E.H. Kennard, Phys. Rev. **29**, 466 (1927).

[5] B.I. Stepanov, Doklady Akademii Nauk SSSR **112**, 839 (1957).

[6] D.E. McCumber, Phys. Rev. **136**, A954 (1964).

[7] R.T. Ross, J. Chem. Phys. **46**, 4590 (1967).

[8] R.L. van Metter and R.S. Knox, Chem. Phys. **12**, 333 (1976).

[9] J.R. Lakowicz, *Principles of Fluorescence Spectroscopy* (Kluwer Academic, New York, 1999).

[10] P. Würfel, J. Phys. C: Solid State Phys. **15**, 3967 (1982).

[11] M.S. Tomas and Z. Lenac, Phys. Rev. A **56**, 4197 (1997).

[12] M.S. Tomas and Z. Lenac, Phys. Rev. A **60**, 2431 (1999).

[13] Y. Lee and M. Yamanishi, Phys. Rev. A **52**, 2312 (1995).

[14] H. Yokoyama and S.D. Brorson, J. Appl. Phys. **66**, 4801 (1989).

[15] E. de Angelis, F. de Martini, and P. Mataloni, J. Opt. B **2**, 149 (2000).

[16] M. Djiango, T. Kobayashi, and W. J. Blau, Appl. Phys. Lett. **93**, 143306 (2008).

[17] A.J. Campillo, J.D. Eversole, and H-B. Lin, Phys. Rev. Lett. **67**, 437 (1991).

[18] L. Andreani, G. Panzarini, and J.-M. Gerard, Phys. Rev. B **60**, 13276 (1999).

[19] J. Klaers, J. Schmitt, F. Vewinger, and M. Weitz, Nature **468**, 545 (2010).

[20] J. Klaers, F. Vewinger, and M. Weitz, Nature Phys. **6**, 512 (2010).

[21] J. Klaers, J. Schmitt, T. Damm, F. Vewinger, and M. Weitz, Appl. Phys. B **105**, 17 (2011)

[22] E.B. Rockover, N.B. Abraham, and S.R. Smith, Phys. Rev. A **17**, 1100 (1978)
